# Supplementary material for: KorMedMCQA: Multi-Choice Question Answering Benchmark for Korean Healthcare Professional Licensing Examinations
Source: arXiv:2403.01469 source file (2024-12-09)
Supplement: Supplementary file 2 [file table11.tex]

\begin{tabular}{llcccccccccc}
\toprule
\multicolumn{1}{l}{\textbf{Model}} & \multicolumn{1}{l}{\textbf{Citation}} & \multicolumn{1}{c}{\textbf{Doctor}} & \multicolumn{1}{c}{\textbf{Nurse}} & \multicolumn{1}{c}{\textbf{Pharm}} & \multicolumn{1}{c}{\textbf{Dentist}} & \multicolumn{1}{c}{\textbf{Avg}} & \multicolumn{1}{c}{\textbf{MedQA}} & \multicolumn{1}{c}{\textbf{IFEval}} & \multicolumn{1}{c}{\textbf{BBH}} & \multicolumn{1}{c}{\textbf{GPQA}} & \multicolumn{1}{c}{\textbf{MMLU-PRO}} \\ 
\midrule
\multicolumn{12}{c}{\textbf{Human Performance}}  \\ \midrule
Examinees Average&&79.66&79.90&71.86&78.23&77.05&-&-&-&-&- \\
\midrule 

\multicolumn{12}{c}{\textbf{Proprietary Models}}                                                                                                                                       \\ \midrule
o1-preview-2024-09-12 & \citet{openai2024b} & 92.41 & 95.10 & 94.24 & 88.66 & \textbf{92.72} & 94.19 &-&-&-&- \\
o1-mini-2024-09-12 & \citet{openai2024b} & 88.28 & 85.88 & 87.68 & 69.91 & 82.45 & 90.18 &-&-&-&- \\
gpt-4o-2024-08-06 & \citet{openai2024a} & 85.98 & 91.46 & 85.99 & 78.67 & 85.61 & 86.96 &-&-&-&- \\
gpt-4o-mini-2024-07-18 & \citet{openai2024a} & 63.22 & 83.14 & 71.30 & 59.06 & 70.29 & 72.90 &-&-&-&- \\
gpt-4-turbo-2024-04-09 & \citet{achiam2023gpt} & 76.32 & 86.67 & 81.02 & 66.71 & 78.13 & 76.43 &-&-&-&- \\
gpt-4-0125-preview & \citet{achiam2023gpt} &75.17 & 86.90 & 81.92 & 66.46 & 78.23 & 78.24 &-&-&-&- \\
gpt-3.5-turbo-0125 & \citet{brown2020language} & 31.26 & 52.85 & 46.55 & 32.06 & 42.27 & 78.55 &-&-&-&- \\
claude-3-5-sonnet-20241022&\citet{anthropic2024b}&88.05&92.14&91.41&74.23&86.51 & 82.95 &-&-&-&- \\
claude-3-5-haiku-20241022&\citet{anthropic2024b}&69.66&81.89&58.42&62.27&67.93 & 69.21 &-&-&-&- \\
claude-3-opus-20240229&\citet{anthropic2024a}&74.25&87.24&74.35&69.30&76.74 & 76.12 &-&-&-&- \\
claude-3-sonnet-20240229&\citet{anthropic2024a}&66.90&78.13&63.73&43.25&62.87 & 65.91 &-&-&-&- \\
gemini-1.5-pro&\citet{team2024gemini}&79.31&88.27&80.34&70.28&79.79 & 76.67 &-&-&-&- \\
gemini-1.5-flash&\citet{team2024gemini}&68.51&82.46&74.92&59.68&72.09 & 67.09 &-&-&-&- \\
\midrule

\multicolumn{12}{c}{\textbf{Multilingual Models}}                                                                                                                    \\ \midrule
Llama-3.1-70B-Instruct&\citet{dubey2024llama}&72.18&82.23&77.74&63.13&74.31&79.42&86.69&55.93&14.21&47.88 \\
Llama-3.1-8B-Instruct&\citet{dubey2024llama}&40.69&59.57&55.25&42.05&50.85&63.32&78.56&29.89&2.35&30.68 \\
Llama-3-70B-Instruct&\citet{dubey2024llama}&66.67&81.21&73.90&63.01&72.05&75.88&80.99&50.19	&4.92	&46.74 \\
Llama-3-8B-Instruct&\citet{dubey2024llama}&38.16&55.92&48.14&41.68&47.23&62.37&74.08&	28.24&	1.23&	29.6 \\
Llama-2-70b-chat-hf&\citet{touvron2023llama}&28.51&45.67&38.08&31.69&37.19&50.75&49.58	&4.61	&1.9&	15.92 \\
Llama-2-13b-chat-hf&\citet{touvron2023llama}&27.36&36.67&31.41&30.83&32.20&42.81&39.85&	7.16&	0&	10.26 \\
Llama-2-7b-chat-hf&\citet{touvron2023llama}&21.61&27.45&25.42&25.77&25.56&38.81&39.86	&4.46&	0.45	&7.64 \\
Qwen2.5-72B-Instruct&\citet{yang2024qwen2}&77.24&87.47&82.71&66.21&\textbf{78.86}&77.93&86.38&61.87&16.67&51.40 \\
Qwen2.5-7B-Instruct&\citet{yang2024qwen2}&51.49&27.33&63.39&39.58&44.73&61.19&75.85&34.89&5.48&36.52 \\
Qwen2.5-1.5B-Instruct&\citet{yang2024qwen2}&33.33&47.72&35.48&32.43&37.92&45.56&44.76&19.81&0.78&19.99 \\
Qwen2-72B-Instruct&\citet{yang2024qwen2}&74.71&86.90&82.03&68.68&78.79&75.41&79.89&57.48&16.33&48.92 \\
Qwen2-7B-Instruct&\citet{yang2024qwen2}&46.21&66.86&57.85&44.27&55.14&55.30&56.79&37.81&6.38&31.64 \\
Qwen2-1.5B-Instruct&\citet{yang2024qwen2}&28.97&44.65&32.54&27.87&34.30&39.67&33.71	&13.7&1.57&16.68 \\
Mistral-Large-Instruct-2411&\citet{mistral2024}&71.26&82.46&78.64&62.89&74.44&79.81&84.01&52.74&24.94&50.69 \\
Mistral-Large-Instruct-2407&\citet{mistral2024}&71.49&83.83&80.45&62.89&75.41&79.65&-&-&-&- \\
Mistral-Nemo-Instruct-2407&\citet{mistral2024}&42.30&65.83&58.31&43.03&54.07&60.88&63.80&29.68&5.37&27.97 \\
Mixtral-8x22B-Instruct-v0.1&\citet{jiang2024mixtral}&48.28&69.36&66.44&47.84&59.65&69.91&71.84&44.11&16.44&38.7 \\
Mixtral-8x7B-Instruct-v0.1&\citet{jiang2024mixtral}&36.55&56.95&54.80&38.84&48.49&61.19&55.99&29.74&7.05&29.91 \\
Mistral-7B-Instruct-v0.3&\citet{jiang2023mistral}&29.66&42.37&41.13&31.20&37.16&51.37 &54.65&25.57&3.91&23.06\\
gemma-2-27b-it&\citet{team2024gemmab}&62.30&78.36&72.20&58.57&68.89&67.79&79.78&49.27&16.67&38.35 \\
gemma-2-9b-it&\citet{team2024gemmab}&20.69&61.73&43.95&42.42&45.36&62.53&74.36&42.14&14.77&31.95 \\
gemma-2-2b-it&\citet{team2024gemmab}&13.33&39.41&27.80&28.11&29.18&42.18&56.68&17.98&3.24&17.22 \\
gemma-7b-it&\citet{team2024gemmaa}&28.89&41.80&34.35&29.96&34.70&39.67&38.68&11.88&4.59&7.72 \\
gemma-1.1-2b-it&\citet{team2024gemmaa}&22.30&25.17&22.60&22.32&23.23&28.99&30.67&5.86&2.57&5.37 \\
Yi-1.5-34B-Chat&\citet{young2024yi}&36.09&51.03&48.81&38.84&44.93&63.55&60.67&44.26&15.32&39.12 \\
Yi-1.5-9B-Chat&\citet{young2024yi}&31.26&44.99&38.98&34.77&38.48&52.24&60.46&36.95&11.3&33.06 \\
Yi-34B-Chat&\citet{young2024yi}&33.33&53.30&50.62&38.72&45.70&63.63&46.99&37.62&11.74&34.37 \\
Yi-6B-Chat&\citet{young2024yi}&28.28&33.49&37.85&29.59&32.97&48.70&33.95&17&5.93&22.9 \\
Phi-3.5-mini-instruct&\citet{abdin2024phi}&34.25&49.66&44.29&37.48&42.57&48.78&57.75&36.75&11.97&32.91 \\
Phi-3.5-MoE-instruct&\citet{abdin2024phi}&52.64&76.08&67.23&52.40&63.71&70.52&69.25&48.77&14.09&40.64 \\
Phi-3-mini-4k-instruct&\citet{abdin2024phi}&29.43&33.37&32.09&27.13&30.74&59.07&54.77&36.56&10.96&33.58 \\
Phi-3-medium-4k-instruct&\citet{abdin2024phi}&31.03&46.47&46.21&35.39&41.18&69.76&64.23&49.38&11.52&40.84 \\
SOLAR-10.7B-Instruct&\citet{kim2023solar}&41.84&58.54&52.77&37.85&48.85&54.52&47.37&31.87&7.83&23.76 \\
\midrule
\multicolumn{12}{c}{\textbf{Korean Specific Models}}                                                                                                                  \\ \midrule
EEVE-Korean-Instruct-10.8B-v1.0&\citet{kim2024efficient}&48.97&66.17&58.19&42.42&54.94&53.50&-&-&-&- \\
EXAONE-3.0-7.8B-Instruct&\citet{an2024exaone}&48.28&67.65&56.61&45.87&55.73&50.59&71.93&17.98&2.13&28.63 \\
KULLM3 & \citet{kullm} & 39.54 & 60.02 & 52.09 & 38.35 & 48.89 & 52.47 & - & - & - & - \\
\midrule
\multicolumn{12}{c}{\textbf{Medical Continual Pretrained \& Finetuned Models}}                                                                                                                      \\ \midrule
Meditron3-70B&\citet{chen2023meditron}&70.57&82.69&75.82&62.64&73.51&79.65&-&-&-&- \\
Meditron3-8B&\citet{chen2023meditron}&38.39&58.20&54.92&39.83&49.42&61.98&-&-&-&- \\
meditron-70b&\citet{chen2023meditron}&42.07&56.61&48.36&37.98&47.06&60.02&-&-&-&- \\
meditron-7b&\citet{chen2023meditron}&24.37&26.20&27.12&24.04&25.62&37.63&-&-&-&- \\
llama-3-meerkat-70b-v1.0&\citet{kim2024small}&69.20&80.75&75.59&60.06&71.99&77.85&-&-&-&- \\
llama-3-meerkat-8b-v1.0&\citet{kim2024small}&38.62&56.61&45.65&40.57&46.46&62.53&-&-&-&- \\
meerkat-7b-v1.0&\citet{kim2024small}&35.17&45.44&44.18&33.66&40.41&61.51&-&-&-&- \\
ClinicalCamel-70B&\citet{toma2023clinical}&43.35&65.15&53.90&42.54&52.61&59.62&-&-&-&- \\
Palmyra-Med-70B&\citet{kamble2023palmyra}&66.67&79.27&73.45&61.65&70.99&77.93&-&-&-&- \\
BioMistral-7B&\citet{labrak2024biomistral}&27.82&37.24&36.16&26.63&32.70&44.38 &-&-&-&-
\\
     \bottomrule
\end{tabular}
