# Supplementary material for: KorMedMCQA: Multi-Choice Question Answering Benchmark for Korean Healthcare Professional Licensing Examinations
Source: arXiv:2403.01469 source file (2024-12-09)
Supplement: Supplementary file 6 [file table3.tex]

\begin{tabular}{l}
\toprule
\textbf{질문:} 13개월 남아가, 형이 하루 전 홍역으로 진단을 받아서 병원에 왔다. 평소 건강하며 현재 특별한 증상은 없다. 맥박 100회/분, 호흡 28회/분, 체온 36.7℃이다. 예방접종 기록은 다음과 같다. 조치는? BCG 1회B형간염백신 3회 DTaP-폴리오-Hib 혼합백신 3회 폐렴구균단백결합백신 4회 일본뇌염백신 1회 \\
\textbf{보기:} A. 경과관찰 B. 비타민A C. 단클론항체 D. 면역글로불린 E. 홍역- 볼거리- 풍진 백신 \\
\textbf{정답:} 차근차근 생각해봅시다. 13개월 남아는 아직 면역체계가 완전히 발달하지 않았으며, 형이 하루 전에 홍역으로 진단을 받았기 때문에 홍역 노출 가능성이 있습니다. 홍역은 전염성이 매우 강하며, 예방접종을 통해 예방이 가능합니다. 예방접종 기록을 살펴보면, BCG, B형간염백신, DTaP-폴리오-Hib 혼합백신, 폐렴구균단백결합백신, 일본뇌염백신이 접종되었으나 홍역-볼거리-풍진(MMR) 백신은 아직 접종되지 않았습니다. 그에 따라,이 아이는 아직 홍역에 대한 면역이 형성되지 않았을 가능성이 높습니다. 홍역 백신 미접종자에게 홍역 노출 후 빠르게 면역을 형성하기 위해 72시간 내 MMR 백신을 접종하는 것이 적절한 조치입니다. 따라서, 정답은 (E) 입니다. \\
\break
\textbf{질문:} 55세 여자가 2일 전부터 열이 난다며 병원에 왔다. 며칠 전부터 평소보다 소변을 자주 본다고 한다. 1개월 전에도 비슷한 증상이 있었다고 한다. 혈압 130/80 mmHg, 맥박 105회/분, 호흡 18회/분, 체온 38.5℃이다. 왼쪽 갈비척추각에 압통이 있다. 소변검사 결과는 다음과 같다. 가능성이 높은 원인미생물은? 백혈구 10～20/고배율시야, 적혈구 0～5/고배율시야 \\
\textbf{보기:} A. 대장균(Escherichia coli ) B. 창자알균(Enterococcus faecalis) C. 프로테우스미라빌리스(Proteus mirabilis) D. 우레아플라스마우레알리티쿰(Ureaplasma urealyticum ) E. 스타필로코쿠스사프로피티쿠스(Staphylococcus saprophyticus) \\
\textbf{정답:} 차근차근 생각해봅시다. 55세 여자는 2일 전부터 열이 나고, 소변을 자주 보는 증상이 있습니다. 또한 왼쪽 갈비척추각에 압통이 있으며, 체온이 38.5℃로 발열이 동반되고 있습니다. 이 환자는 소변검사에서 백혈구가 많이 검출되어 요로감염의 가능성이 높습니다. 특히, 1개월 전에도 비슷한 증상이 있었다고 하므로, 반복적인 요로감염의 가능성도 고려해야 합니다. 요로감염의 주요 원인균은 대장균(Escherichia coli)입니다. 대장균은 요로감염의 가장 흔한 원인균으로, 특히 여성에서 빈번하게 발생합니다. 환자의 소변검사 결과와 임상 증상을 종합해 볼 때, 가장 가능성이 높은 원인 미생물은 대장균입니다. 따라서, 정답은 (A) 입니다. \\
\break
\textbf{질문:} 8세 남아가 쉽게 짜증을 내고 친구를 자주 때려 병원에 왔다. 학교에서는 선생님의 지시를 따르지 못하고 집에서 자주 울고 떼를 썼으며 밤늦게까지 안 자서 엄마가 감당하기 힘들었다. 5세 때 한 차례 경련을 했고 이후로 괜찮아 치료를 받지 않았다. 지능지수는 49이다. 치료는? \\
\textbf{보기:} A. 졸피뎀 B. 도네페질 C. 리스페리돈 D. 아고멜라틴 E. 알프라졸람 \\
\textbf{정답:} 차근차근 생각해봅시다. 8세 남아는 쉽게 짜증을 내고 공격적인 행동을 보이며, 학교와 가정에서 문제를 일으키고 있습니다. 또한, 밤늦게까지 잠을 자지 못해 엄마가 감당하기 어려운 상태입니다. 이 아이는 현재 지능지수는 49로 지적장애가 있는 것으로 보입니다. 이러한 행동 문제는 지적장애와 관련된 행동 장애의 일부일 수 있으며, 치료가 필요합니다. 지적장애와 관련된 행동 장애의 치료는 행동치료, 항정신병 약물 등이 있고 또한 ADHD와의 감별이 필요합니다. 이중 보기에 있는 리스페리돈은 항정신병 약물로, 특히 공격적인 행동이나 자해 등의 문제 행동을 줄이는 데 사용될 수 있습니다. 이 약물은 지적장애가 있는 아이들의 행동 문제를 완화시키는 데 효과적입니다. 따라서, 이 경우 적절한 치료는 리스페리돈이 될 것입니다. 따라서, 정답은 (C) 입니다. \\
\break
\textbf{질문:} 50세 남자가 10일 전부터 서서히 배가 불러온다고 병원에 왔다. 누나와 형이 간질환으로 약을 복용 중이라고 한다. 혈압 110/70 mmHg, 맥박 80회/분, 호흡 18회/분, 체온 36.7℃이다. 결막은 창백하고 공막에 황달이 있다. 앞가슴에 거미혈관종이 보인다. 복부는 팽만하고 이동둔탁음이 있다. 복부에 압통이나 반동압통은 없다. 양쪽 정강뼈앞 오목부종이 있다. 검사 결과는 다음과 같다. 복부 컴퓨터단층촬영 사진이다. 치료는? 혈액: 백혈구 4,700/mm\^3, 혈색소 10.4 g/dL, 혈소판 59,000/mm\^3 프로트롬빈시간(INR) 2.1, 알부민 1.8 g/dL,총빌리루빈 4.2 mg/dL, 아스파르테이트아미노전달효소 69 U/L 알라닌아미노전달효소 18 U/L HBsAg (+), anti-HBs (-), anti-HCV (-) 알파태아단백질 3.9 ng/mL (참고치, <8.5) 복수: 총단백질 1.2 g/dL, 알부민 0.4 g/dL,백혈구 100/mm\^3, 아데노신탈아미노효소(ADA) 9 U/L \\
\textbf{보기:} A. 리팜핀 B. 세포탁심 C. 락툴로오스 D. 스피로놀락톤 E. 메트로니다졸 \\
\textbf{정답:} 차근차근 생각해봅시다. 50세 남자는 10일 전부터 배가 불러오는 증상으로 병원에 왔습니다. 환자의 가족력에서 간질환이 있으며, 현재 환자에게 결막 창백, 황달, 거미혈관종, 복부 팽만, 이동둔탁음, 그리고 오목부종과 같은 간경변의 징후들이 보입니다. 검사 결과에서 저알부민혈증, 고빌리루빈혈증, 그리고 혈소판 감소증이 나타나고 있으며, HBsAg 양성으로 B형 간염과 관련된 만성 간질환이 있을 가능성이 높습니다. 복수 검사 결과, 저단백질 복수와 저알부민 농도가 확인되었습니다. 또한, 복수의 백혈구 수치가 낮아 감염의 가능성이 낮으며, ADA 수치도 결핵성 복수를 시사하지 않습니다. 이러한 소견은 간경변으로 인한 복수의 발생을 의미하며, 이로 인해 복수 관리가 필요합니다. 이 상황에서는 이뇨제인 스피로놀락톤이 복수를 조절하는 데 가장 효과적인 치료법이 될 수 있습니다. 따라서, 정답은 (D) 입니다. \\
\break
\textbf{질문:} 35세 여자가 2주 전부터 배가 불러온다며 병원에 왔다. 2개월 동안 체중이 4 kg 줄었다고 한다. 혈압 110/70 mmHg, 맥박 97회/분, 호흡 21회/분, 체온 38.1℃이다. 의식은 명료하다. 배는 팽만하고 이동둔탁음이 있다. 배에 가벼운 압통은 있으나 반동압통은 없다. 검사 결과는 다음과 같다. 원인은?혈액: 혈색소 11.2g/dL, 백혈구 4,200/mm\^3, 혈소판 169,000/mm\^3 총단백질 6.0 g/dL, 알부민 3.3 g/dL, 총빌리루빈 1.2 mg/dL, 아스파르테이트아미노전달효소 34 U/L 알라닌아미노전달효소 21 U/L 아밀라아제 61 U/L, 리파제 30 U/L 복수: 백혈구 1,500/mm\^3 (중성구 5\%, 림프구 90\%) 단백질 3.1 g/dL, 알부민 2.5 g/dL,아데노신탈아미노효소(ADA) 85 U/L 소변: 단백질 (-), 적혈구 0～2/고배율시야 \\
\textbf{보기:} A. 간경화증 B. 복막결핵 C. 콩팥증후군 D. 급성이자염 E. 복막암종증 \\
\textbf{정답:} 차근차근 생각해봅시다. 35세 여자는 2주 전부터 배가 불러오는 증상으로 병원에 왔고, 최근 2개월 동안 체중이 4 kg 줄어들었습니다. 체온이 38.1℃로 발열이 동반되었고, 복부 팽만과 이동둔탁음이 있습니다. 검사 결과를 보면, 혈액 검사에서 총단백질과 알부민 수치는 정상 하한선에 가깝지만, 복수에서 단백질과 알부민 수치가 상대적으로 높고, ADA(아데노신탈아미노효소) 수치가 85 U/L로 상승되어 있습니다. 복수의 백혈구 수치도 증가했으며 림프구 비율이 높습니다. 이러한 소견들은 결핵에 의한 복막염, 즉 복막결핵을 강력히 시사합니다. ADA 수치의 상승은 특히 결핵성 복막염에서 흔히 관찰됩니다. 따라서, 정답은 (B) 입니다. \\
\bottomrule
\end{tabular}
