# Supplementary material for: KorMedMCQA: Multi-Choice Question Answering Benchmark for Korean Healthcare Professional Licensing Examinations
Source: arXiv:2403.01469 source file (2024-12-09)
Supplement: Supplementary file 8 [file table5.tex]

\begin{tabular}{l}
\toprule
\textbf{질문:} 옥시토신 유도분만 중인 40주 초산부가 통증을 호소하여 사정한 결과는 다음과 같다. 우선적인 간호중재는?• 자궁경관: 개대 2 cm, 소실 70\% • 자궁수축: 간격 2분 미만, 기간 90초 이상, 강도 100 mmHg \\
\textbf{보기:} A. 관장 시행 B. 양막절개술 실시 C. 자궁근이완제 투여 D. 옥시토신 투여 중단 E. 프로스타글란딘 질정 투여 \\
\textbf{정답:} 차근차근 생각해봅시다. 40주 초산부가 옥시토신 유도분만 중에 있습니다. 현재 자궁경관의 개대는 2 cm, 소실은 70\%이며, 자궁수축 간격은 2분 미만이고, 수축 기간은 90초 이상입니다. 강도는 100 mmHg로 매우 강한 상태입니다. 이 경우 자궁수축이 과도하여 태아와 산모에게 위험이 될 수 있습니다. 옥시토신은 자궁수축을 유도하기 위해 사용되지만, 과도한 수축은 자궁의 혈류를 감소시켜 태아의 산소 공급에 영향을 줄 수 있습니다. 현재 이 산모의 자궁수축이 과도하므로, 옥시토신 투여를 중단하거나 감량하는 것이 필요합니다. 따라서, 정답은 (D) 입니다. \\
\break
\textbf{질문:} 심부전 환자의 사정결과가 다음과 같을 때 우선적인 중재는?• 허약, 심한 피로, 야뇨 • 거품이 있는 분홍빛의 객담, 기좌호흡 • 맥박 110회/분, 호흡 30회/분 \\
\textbf{보기:} A. 수분섭취 권장 B. 산소포화도 측정 C. 객담배양검사 실시 D. 트렌델렌부르크자세 유지 E. 복도 걷기와 같은 활동 격려 \\
\textbf{정답:} 차근차근 생각해봅시다. 심부전 환자의 사정 결과를 보면, 허약과 심한 피로, 야뇨가 있으며, 거품이 있는 분홍빛의 객담과 기좌호흡이 나타나고 있습니다. 또한, 맥박은 110회/분, 호흡은 30회/분으로 빈맥과 빈호흡이 관찰됩니다. 이러한 증상들은 폐에 액체가 축적되어 발생하는 폐부종을 시사합니다. 폐부종은 산소 공급에 심각한 영향을 미칠 수 있으며, 즉각적인 중재가 필요합니다. 이 환자의 경우 산소 공급이 필요할 수 있으므로, 우선 산소포화도를 측정하여 산소 요구량을 평가하는 것이 중요합니다. 따라서, 정답은 (B) 입니다. \\
\break
\textbf{질문:} 호흡곤란으로 입원한 환자의 사정결과가 다음과 같을 때 우선적인 중재는?• 3개월 전 승모판대치술을 받음• 목정맥 팽창, 체중 증가• 심박출률(EF) 45\%, 산소포화도 86\% • 혈압 90/60 mmHg, 맥박 102회/분, 호흡 26회/분, 체온 37.5℃ \\
\textbf{보기:} A. 산소 투여 B. 배변완화제 투여 C. 중등도 활동 격려 D. 혈액배양검사 실시 E. 비위관 영양 공급 \\
\textbf{정답:} 차근차근 생각해봅시다. 환자는 3개월 전 승모판대치술을 받은 상태이며, 현재 호흡곤란으로 입원 중입니다. 사정결과를 보면 목정맥 팽창과 체중 증가가 나타나고 있으며, 심박출률(EF)이 45\%로 감소한 상태입니다. 또한, 산소포화도가 86\%로 저하되어 있고, 혈압은 90/60 mmHg로 낮으며, 맥박과 호흡도 증가한 상태입니다. 이 환자의 상황은 심부전의 증상으로 볼 수 있으며, 특히 산소포화도가 86\%로 낮은 상태는 산소 공급이 부족함을 의미합니다. 즉각적인 산소 공급이 필요할 수 있으므로, 우선 산소를 투여하는 것이 중요합니다. 따라서, 정답은 (A) 입니다. \\
\break
\textbf{질문:} 외래 진료를 받고 있는 환자의 사정결과가 다음과 같을 때 간호중재는? • 전신 소양증, 만성 두통• 적혈구 800만/mm\^3, 헤모글로빈 20 g/dL,헤마토크리트 60\%, 혈소판 45만/mm\^3 \\
\textbf{보기:} A. 침상안정을 한다. B. 철분제제를 투여한다. C. 치실을 사용하여 치아를 관리한다. D. 앉아있을 때 다리를 내리도록 한다. E. 수분을 하루 3 L 이상 섭취하도록 격려한다. \\
\textbf{정답:} 차근차근 생각해봅시다. 외래 진료를 받고 있는 환자의 사정 결과를 보면 전신 소양증과 만성 두통을 호소하고 있으며, 혈액 검사 결과 적혈구 수치가 800만/mm³로 매우 높고, 헤모글로빈이 20 g/dL, 헤마토크리트가 60\%로 증가되어 있습니다. 혈소판 수치도 45만/mm³로 높게 나타났습니다. 이러한 결과는 적혈구 증가증(polycythemia)를 시사하며, 이는 혈액이 끈적해지고 혈전 발생 위험이 증가할 수 있는 상태입니다. 혈액의 점도를 낮추고 혈액 순환을 원활하게 하기 위해서는 충분한 수분 섭취가 필요합니다. 따라서, 이 환자에게는 수분을 하루 3L 이상 섭취하도록 격려하는 것이 중요합니다. 따라서, 정답은 (E) 입니다. \\
\break
\textbf{질문:} 패혈증 환자의 사정결과가 다음과 같을 때 우선적인 중재는?• 심한 호흡곤란, 의식수준 저하, 창백한 피부• 맥박 110회/분, 수축기 혈압 70 mmHg • 흉부 X선 검사 시 양쪽 폐 부위가 하얗게 나타남• 동맥혈가스분석: 이산화탄소분압 70 mmHg 산소분압 50 mmHg, pH 7.18산소포화도 65\% \\
\textbf{보기:} A. 비위관 삽입 B. 항응고제 투여 C. 인공호흡기 적용 D. 폐기능검사 실시 E. 흉부물리요법 제공 \\
\textbf{정답:} 차근차근 생각해봅시다. 이 환자는 패혈증으로 인해 심한 호흡곤란과 의식수준 저하, 창백한 피부를 보이고 있습니다. 맥박은 110회/분으로 빈맥이 나타나고 있으며, 수축기 혈압이 70 mmHg로 매우 낮은 상태입니다. 흉부 X선 검사에서는 양쪽 폐 부위가 하얗게 나타나, 폐에 심각한 이상이 있음을 시사합니다. 또한, 동맥혈가스분석 결과 이산화탄소분압이 70 mmHg로 상승하고, 산소분압이 50 mmHg로 저하되어 있으며, pH는 7.18로 산증 상태입니다. 산소포화도는 65\%로 매우 낮아, 환자는 심각한 저산소증 상태에 있습니다. 이 상황에서는 즉각적인 산소 공급이 필수적이며, 환자가 자발적으로 호흡을 유지하기 어려운 상태이므로 인공호흡기를 적용하여 산소를 공급하고 환자의 호흡을 보조하는 것이 필요합니다. 따라서, 정답은 (C) 입니다. \\
\bottomrule
\end{tabular}
