# Supplementary material for: KorMedMCQA: Multi-Choice Question Answering Benchmark for Korean Healthcare Professional Licensing Examinations
Source: arXiv:2403.01469 source file (2024-12-09)
Supplement: Supplementary file 12 [file table9.tex]

\begin{tabular}{l}
\toprule
\textbf{질문:} 국소의치에서 하중부담을 고려하여 최종인상을 채득할 때, 왁스 릴리프의 양을 최대로 확보해야 하는 부위는? \\
\textbf{보기:} A. 절치유두 B. 협측 선반 C. 상악 치조정 D. 상악 치조제의 협측 경사면 E. 하악 치조제의 설측 경사면 \\
\textbf{정답:} 차근차근 생각해봅시다. 국소의치에서 하중부담을 고려하여 최종인상을 채득할 때, 왁스 릴리프의 양을 최대로 확보해야 하는 부위를 선택해야 합니다. 왁스 릴리프는 압박이 가해지는 부위를 보호하고 환자의 불편감을 줄이기 위해 필요합니다. 절치유두는 상악에서 특히 압박을 받을 수 있는 부위로, 이곳에 적절한 완충을 제공하는 것이 중요합니다. 따라서, 이 부위에 왁스 릴리프를 최대한으로 확보해야 합니다. 따라서, 정답은 (A) 입니다. \\
\break
\textbf{질문:} 후방연장 의치상의 지지를 얻기 위해 이차인상을 이용하여 개조모형(altered cast)을 만드는 것이 추천되는 부분무치악 분류는? \\
\textbf{보기:} A. 상악 Kennedy Class I B. 하악 Kennedy Class I C. 상악 Kennedy Class II D. 하악 Kennedy Class III E. 하악 Kennedy Class IV \\
\textbf{정답:} 차근차근 생각해봅시다. 후방연장 의치는 후방에 지지되는 치아가 없으므로 의치의 안정성을 위해 지지를 잘 확보하는 것이 중요합니다. 개조모형은 이차인상을 통해 보다 정확한 연조직의 상태를 반영하여 의치를 제작할 수 있도록 도와줍니다. 특히 후방연장이 필요한 Kennedy Class I의 경우 양측 후방에 지지 치아가 없기 때문에 이차인상을 통해 개조모형을 만드는 것이 중요합니다. 따라서, 상악과 하악의 Kennedy Class I에서 이 방법이 추천됩니다. 따라서, 정답은 (B) 입니다. \\
\break
\textbf{질문:} 치주-보철을 위한 보조적 교정치료 시 고정식 교정장치 대신 가철식 교정장치를 사용하는 이유는? \\
\textbf{보기:} A. 발음 및 저작장애가 없다. B. 치아 이동 모멘트의 부여가 쉽다. C. 이동부 치아의 효과적인 이동이 가능하다. D. 치료결과가 환자의 협조에 의해 좌우되지 않는다. E. 치아 이외의 조직에서 고정원(anchorage)을 추가로 얻을 수 있다. \\
\textbf{정답:} 차근차근 생각해봅시다. 치주-보철을 위한 보조적 교정치료 시 가철식 교정장치를 선택하는 이유는 주로 환자의 편의성과 특정 치료 목표에 맞춘 조절 가능성 때문입니다. 고정식 교정장치에 비해 가철식 교정장치는 환자가 직접 탈착이 가능하여 일상생활에서 발음 및 저작장애가 적고, 필요할 때만 장치를 착용할 수 있다는 장점이 있습니다. 또한, 가철식 교정장치는 치아 이외의 조직에서 추가적인 고정원을 얻을 수 있어 교정치료 시 효과적인 결과를 얻는 데 도움을 줍니다. 따라서, 정답은 (E) 입니다. \\
\break
\textbf{질문:} 편측성 완전구순구개열 환자의 치조열 이차골이식술을 시행 하기에 가장 선호되는 시기는? \\
\textbf{보기:} A. 1세경 B. 5세경 C. 10세경 D. 15세경 E. 20세경 \\
\textbf{정답:} 차근차근 생각해봅시다. 치조열 이차골이식술은 구순구개열 환자의 치조골 결손을 보충하기 위해 수행되는 중요한 수술입니다. 이 수술은 영구견치의 맹출 시기에 맞추어 시행되는 것이 가장 효과적입니다. 왜냐하면 이 시기에 치조골을 이식하면 견치의 정상적인 맹출을 도울 수 있기 때문입니다. 일반적으로 견치는 9세에서 11세 사이에 맹출하므로, 이식술은 이보다 조금 이른 10세경에 시행하는 것이 이상적입니다. 따라서, 정답은 (C) 입니다. \\
\break
\textbf{질문:} 상악 무치악 구강에서 저작압을 가장 많이 지지할 수 있는 부위는? \\
\textbf{보기:} A. 구개융기 B. 정중구개봉선 C. 경구개 후방부위 D. 경구개의 평탄한 부분 E. 구상절흔(hamular notch) \\
\textbf{정답:} 차근차근 생각해봅시다. 상악 무치악 구강에서 저작압을 가장 많이 지지할 수 있는 부위를 선택해야 합니다. 경구개 후방부위는 해부학적으로 두꺼운 골 구조와 함께 저작압을 잘 견딜 수 있는 조직을 포함하고 있습니다. 이는 상악 무치악에서 저작압의 분산 및 지지를 제공하는 주요 부위로 평가됩니다. 따라서, 정답은 (C) 입니다. \\
\bottomrule
\end{tabular}
