# Supplementary material for: KorMedMCQA: Multi-Choice Question Answering Benchmark for Korean Healthcare Professional Licensing Examinations
Source: arXiv:2403.01469 source file (2024-12-09)
Supplement: Supplementary file 13 [file table1.tex]

\begin{tabular}{c|c|cccc}
\toprule
Split & Year & Doctor & Nurse & Pharm & Dentist \\ \midrule
\multirow{9}{*}{Train} & 2012 & 309 & - & - & - \\
 & 2013 & 257 & - & - & - \\
 & 2014 & 242 & - & - & - \\
 & 2015 & 226 & - & - & - \\
 & 2016 & 203 & - & - & - \\
 & 2017 & 179 & - & - & - \\
 & 2018 & 164 & - & - & - \\
 & 2019 & 163 & 291 & 318 & - \\
 & 2020 & 147 & 291 & 314 & 297 \\ \midrule
Dev & 2021 & 164 & 291 & 300 & 304 \\ \midrule
\multirow{3}{*}{Test} & 2022 & 135 & 295 & 301 & 302 \\
 & 2023 & 150 & 292 & 313 & 257 \\
 & 2024 & 150 & 291 & 271 & 252 \\ \midrule
Total & - & 2,489 & 1,751 & 1,817 & 1,412 \\ \bottomrule
\end{tabular}
