# Supplementary material for: KorMedMCQA: Multi-Choice Question Answering Benchmark for Korean Healthcare Professional Licensing Examinations
Source: arXiv:2403.01469 source file (2024-12-09)
Supplement: Supplementary file 15 [file table_cot_result.tex]

\begin{tabular}{l|ccccc}
\toprule
\textbf{Model} & \textbf{Doctor} & \textbf{Nurse} & \textbf{Pharmacist} & \textbf{Dentist} & \textbf{Average} \\ \midrule
GPT-4o & 85.98 & 91.46 & 85.99 & 78.67 & 85.61 \\
GPT-4o (CoT) & 89.89 & 92.26 & 90.96 & 79.78 & 88.17 \\ \midrule
Claude-3.5-sonnet & 88.05 & 92.14 & 91.41 & 74.23 & 86.51 \\
Claude-3.5-sonnet (CoT) & 92.18 & 93.96 & 93.22 & 84.59 & 90.96 \\ \midrule
Gemini-1.5-pro & 79.31 & 88.27 & 80.34 & 70.28 & 79.79 \\
Gemini-1.5-pro (CoT) & 84.83 & 90.77 & 87.12 & 67.82 & 82.65 \\ \bottomrule
\end{tabular}
